# Supplementary material for: Critical size limits for collinear and spin spiral magnetism in CoCr$_2$O$_4$
Source: arXiv:1908.10582 ancillary file (2019-08-28)
Supplement: Supplementary file 1 [file supplemental.pdf]

# Critical size limits for collinear and spin spiral magnetism in $CoCr_2O_4$

D. Zákutná[1,2], A. Alemayehu[3], J. Vlček[4], K. Nemkovski[5], C. P. Grams[6], D. Nižňanský[3],* D. Honecker[1],† and S. Disch[2‡]

[1]*Institut Laue-Langevin, 71 Avenue des Martyrs, F-38042 Grenoble, France*

[2]*Department für Chemie, Universität zu Köln, Luxemburger Strasse 116, 50939 Köln, Germany*

[3]*Department of Inorganic Chemistry, Faculty of Science, Charles University in Prague, Hlavova 2030/8, 12843 Prague 2, Czech Republic*

[4]*Department of Physics and Measurements, University of Chemistry and Technology Prague, Technicka 5, 16628 Prague, Czech Republic*

[5]*Forschungszentrum Jülich GmbH, Jülich Centre for Neutron Science (JCNS) at Heinz Maier-Leibnitz Zentrum (MLZ), Lichtenbergstr. 1, 85748 Garching, Germany and*

[6] *II. Physikalisches Institut, Universität zu Köln, Zülpicher Str. 77, 50937, Köln, Germany*

(Dated: August 28, 2019)

### A. Experimental

Cobalt chromite NPs were synthesized by a hydrothermal method according to[1]. Water solution of metal chlorides was prepared by dissolving chromium and cobalt chloride hexahydrate in molar ratio ($Cr^{3+}$: $Co^{2+}$ = 2:1), which was added to a water/ethanol (1:1) solution of sodium oleate. The final mixture was transferred into an autoclave with 50 mL teflon liner and heated to 200°C for 16 h. After cooling down, the liquid phases were discarded, and the sedimented nanoparticles were washed three times by dispersing in hexane and precipitating in ethanol in order to remove all remaining free oleic acid and sodium chloride. The six different particle sizes were obtained by annealing the amorphous as-prepared nanoparticles at 300, 350, 400, 450, 500 and 550°C for 2 h. In the following, the samples are labeled with the prefix AA and numbers corresponding to the annealing temperature.

Powder X-ray diffraction (PXRD) was performed using a PANalytical X'Pert PRO diffractometer with Cu $K_\alpha$ radiation ($\lambda = 1.54$ Å). The diffractometer is equipped with a PIXcel detector and a secondary monochromator. The samples were measured in the $2\theta$-range of 5 - 80 ° with a step size of 0.003 °. The instrumental broadening was obtained with a $LaB_6$ reference (SR 660b, NIST). For the Le-Bail refinement of the diffraction patterns the FullProf software[2] was used.

Transmission Electron Microscopy (TEM) was done in bright field (BF) mode on a ZEISS LEO 902 microscope operating at 120 kV with $LaB_6$ cathode. The samples were deposited onto coated copper grid. The mean particle diameter was statistically determined from at least 200 particles in different BF images and fitted with log-normal size distribution.

Integral magnetization measurements were performed on a Quantum Design Physical Property Measurement System (PPMS) equipped with a superconducting magnet and a vibrating sample magnetometer (VSM) option. The zero-field-cooled (ZFC) and field-cooled (FC) magnetization measurements were done between 2 and 300 K with a heating rate of 1 K/min in an applied magnetic field of $\mu_0 H = 10$ mT. The isothermal, field-dependent magnetization was measured at the base temperature of 2, 10, 30, and above 80 K. AC susceptometry was performed at Quantum Design Physical Property Measurement System (PPMS Evercool) equipped with a superconducting magnet and an ACMSII option. Temperature dependence of the AC field response was determined with AC field amplitude of

0.7 mT at frequencies of 10, 95, 292 and 900 Hz.

Polarized neutron scattering experiments with XYZ polarization analysis were performed at the DNS instrument[3,4] at MLZ in Garching, Germany. Measurements covered a temperature range of 3.2 K -100 K using a neutron wavelength of $\lambda = 4.2$ Å. NiCr and vanadium were used as references for the correction of flipping ratio and detector efficiency, respectively. The magnetic, nuclear coherent and spin-incoherent contributions were separated from the total scattering cross section by means of XYZ-polarization analysis using the 'dnsplot' interface[5].

Measurements of the macroscopic polarization of $CoCr_2O_4$ nanoparticles were performed on a separate part of the sample batches that was slightly pressed and put between capacitor plates. Due to the random orientation of the particles a direct measurement of the polarization is not expected to yield a large signal[6]. Therefore, we applied a static electric field $E_{dc} \approx 1$ kV/mm at temperatures above the expected phase transition and cooled the sample down to 10 K. To orient the particles, we applied magnetic field perpendicular to $E_{dc}$ that was oscillated between 0.1 and -0.1 T at this temperature. After this poling procedure, the electric field was turned off, the sample reheated to 40 K, and the actual temperature dependent measurement was performed on cooling in zero magnetic field to find $T_s$.

## B. Le-Bail Analysis

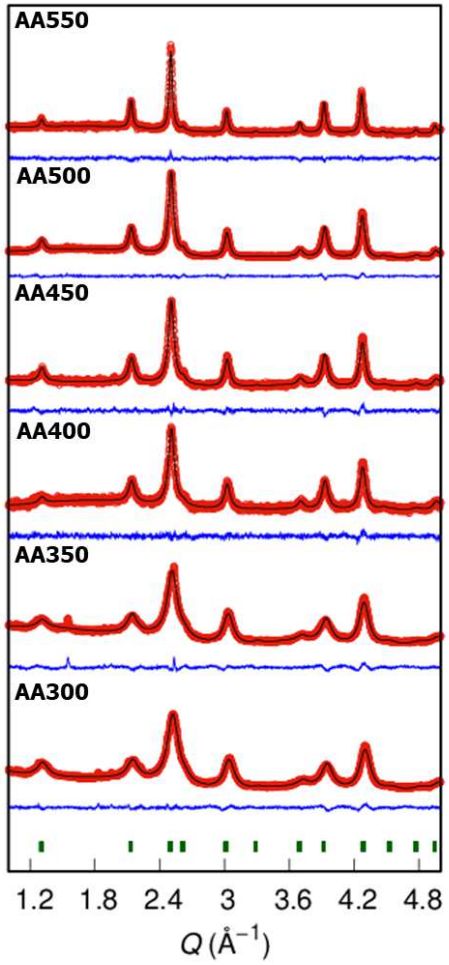


Fig. S 1. Le-Bail analysis (black line) of all prepared samples. Experimental data are presented with red points, residual indicated with blue line and the green vertical lines correspond to the Bragg maxima of spinel structure. The numbers in the sample name indicate the annealing temperature.

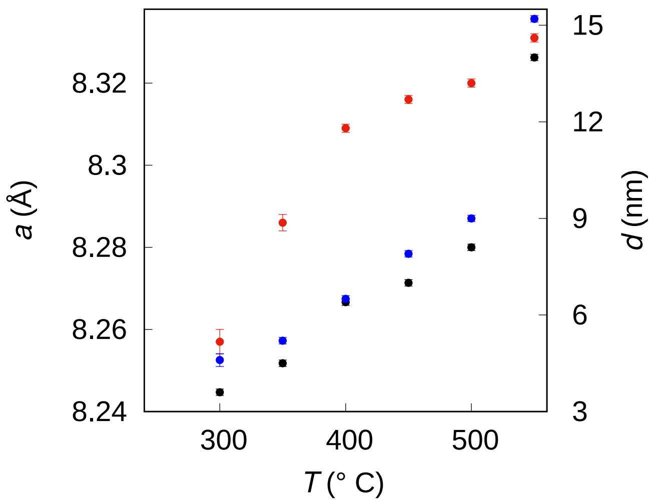


Fig. S 2. Dependence of lattice parameter $a$ (red) and particle size $d_{\mathrm{XRD}}$ (black) and $d_{\mathrm{TEM}}$ (blue points) on the annealing temperature determined from XRD and TEM, respectively. For comparison, the bulk lattice parameter is 8.33 Å[7].

Table S I: Summary of refined Le-Bail parameters with lattice parameter $a$, Lorentzian broadening Y and zero shift.

| **Sample** / **Parameter** | **AA550** | **AA500** | **AA450** | **AA400** | **AA350** | **AA300** |
|---|---|---|---|---|---|---|
| $a$ (Å) | 8.331(1) | 8.320(1) | 8.316(1) | 8.309(1) | 8.286(2) | 8.274(2) |
| **Profile function** | Thompson-Cox-Hastings pseudo-Voigt | | | | | |
| Y (0.01°) | 0.405(4) | 0.661(7) | 0.810(1) | 0.871(1) | 1.732(1) | 2.032(4) |
| zero shift (0.01°) | 0.087(2) | 0.075(1) | 0.089(3) | 0.107(1) | 0.173(1) | 0.047(2) |
| $R_f$ (%) | 0.552 | 0.168 | 0.281 | 0.335 | 0.330 | 0.180 |
| $R_B$ (%) | 0.486 | 0.174 | 0.209 | 0.300 | 0.349 | 0.208 |
| $R_{wp}$ (%) | 6.21 | 2.77 | 6.15 | 6.50 | 3.27 | 2.59 |
| $R_{exp}$ (%) | 6.08 | 2.10 | 5.93 | 6.78 | 1.98 | 1.88 |
| $\chi^2$ | 1.04 | 1.73 | 1.08 | 1.04 | 2.73 | 1.9 |
| **Background function** | Chebyshev polynomial function | | | | | |
| **Refined parameters** | 7 | 9 | 9 | 9 | 9 | 12 |
| **Total fit parameters** | 10 | 12 | 12 | 12 | 12 | 15 |

Table S II: Coherent domain size $d_{\mathrm{XRD}}$ and lattice parameter $a$ obtained from PXRD in comparison to the particle size $d_{\mathrm{TEM}}$ from TEM with size distribution $\sigma_{\mathrm{log}}$. For comparison the bulk lattice parameter 8.33 Å[7].

| **Sample** | $a$ (Å) | $d_{\mathrm{XRD}}$ (nm) | $d_{\mathrm{TEM}}$ (nm) | $\sigma_{\mathrm{log}}$ (%) |
|---|---|---|---|---|
| **AA550** | 8.331(1) | 14.0(1) | 15.2(1) | 17.7(1) |
| **AA500** | 8.320(1) | 8.1(1) | 9.0(1) | 20.0(1) |
| **AA450** | 8.316(1) | 7.0(1) | 7.9(1) | 15.7(1) |
| **AA400** | 8.309(1) | 6.4(1) | 6.5(1) | 13.2(1) |
| **AA350** | 8.286(2) | 4.5(1) | 5.2(1) | 17.0(2) |
| **AA300** | 8.274(2) | 3.6(1) | 4.6(2) | 20.1(2) |

### C. Magnetization measurements

From the frequency dependence of the real part of AC susceptibility, the initial frequency shift is calculated using the formula: $\delta T_{\mathrm{f}} = \Delta T_{\mathrm{f}}/(T_{\mathrm{f}} \Delta log(f))$ yielding values of 0.001, 0.002, 0.002, 0.002 and 0.004 for the samples AA550, AA450, AA400, AA350 and AA300, respectively. The low values of $\delta T_{\mathrm{f}}$ indicate a well-ordered magnetic state.

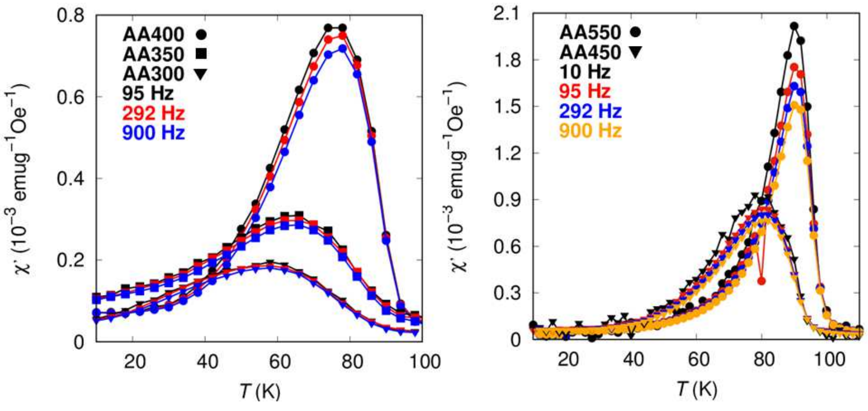


Fig. S 3. Real part of the AC susceptibility of the prepared $CoCr_2O_4$ samples.

Table S III: Summary of the asymptotic Curie temperature $\theta_{\mathbf{C}}$ (from PND and VSM), blocking temperature $T_{\mathbf{b}}$ (from VSM) and spin-spiral transition temperature $T_{\mathbf{s}}$ (from PND).

| **Sample** | $d_{\mathbf{PXRD}}$ (nm) | $\theta_{\mathbf{C,PND}}$ (K) | $\theta_{\mathbf{C,VSM}}$ (K) | $T_{\mathbf{b}}$ (K) | $T_{\mathbf{s}}$ (K) | $M_{\mathbf{s}}$ (50 K) ($\mathrm{Am^{-1}kg^{2}}$) |
|---|---|---|---|---|---|---|
| **AA550** | 14.0(1) | 93(2) | 96(1) | 92(2) | 28(3) | 2.07(3) |
| **AA500** | 8.1(1) | 92(2) | 93(1) | 86(3) | 23(3) | 1.90(3) |
| **AA450** | 7.0(1) | 84(2) | 92(1) | 81(2) | 25(5) | 1.45(2) |
| **AA400** | 6.4(1) | 86(2) | 86(1) | 72(2) | 21(4) | 1.05(5) |
| **AA350** | 4.5(1) | 57(3) | 73(1) | 54(3) | 3.5(3) | 0.74(4) |
| **AA300** | 3.6(1) | - | 56(1) | 44(4) | - | 0.63(1) |

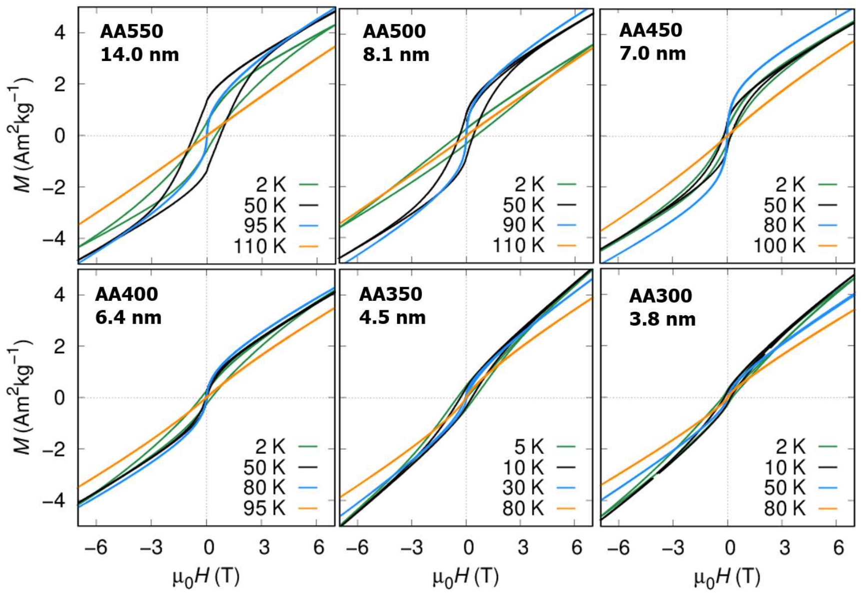


Fig. S 4. Isothermal magnetization of cobalt chromite with different sizes recorded at selected temperatures.

## D. Neutron diffraction

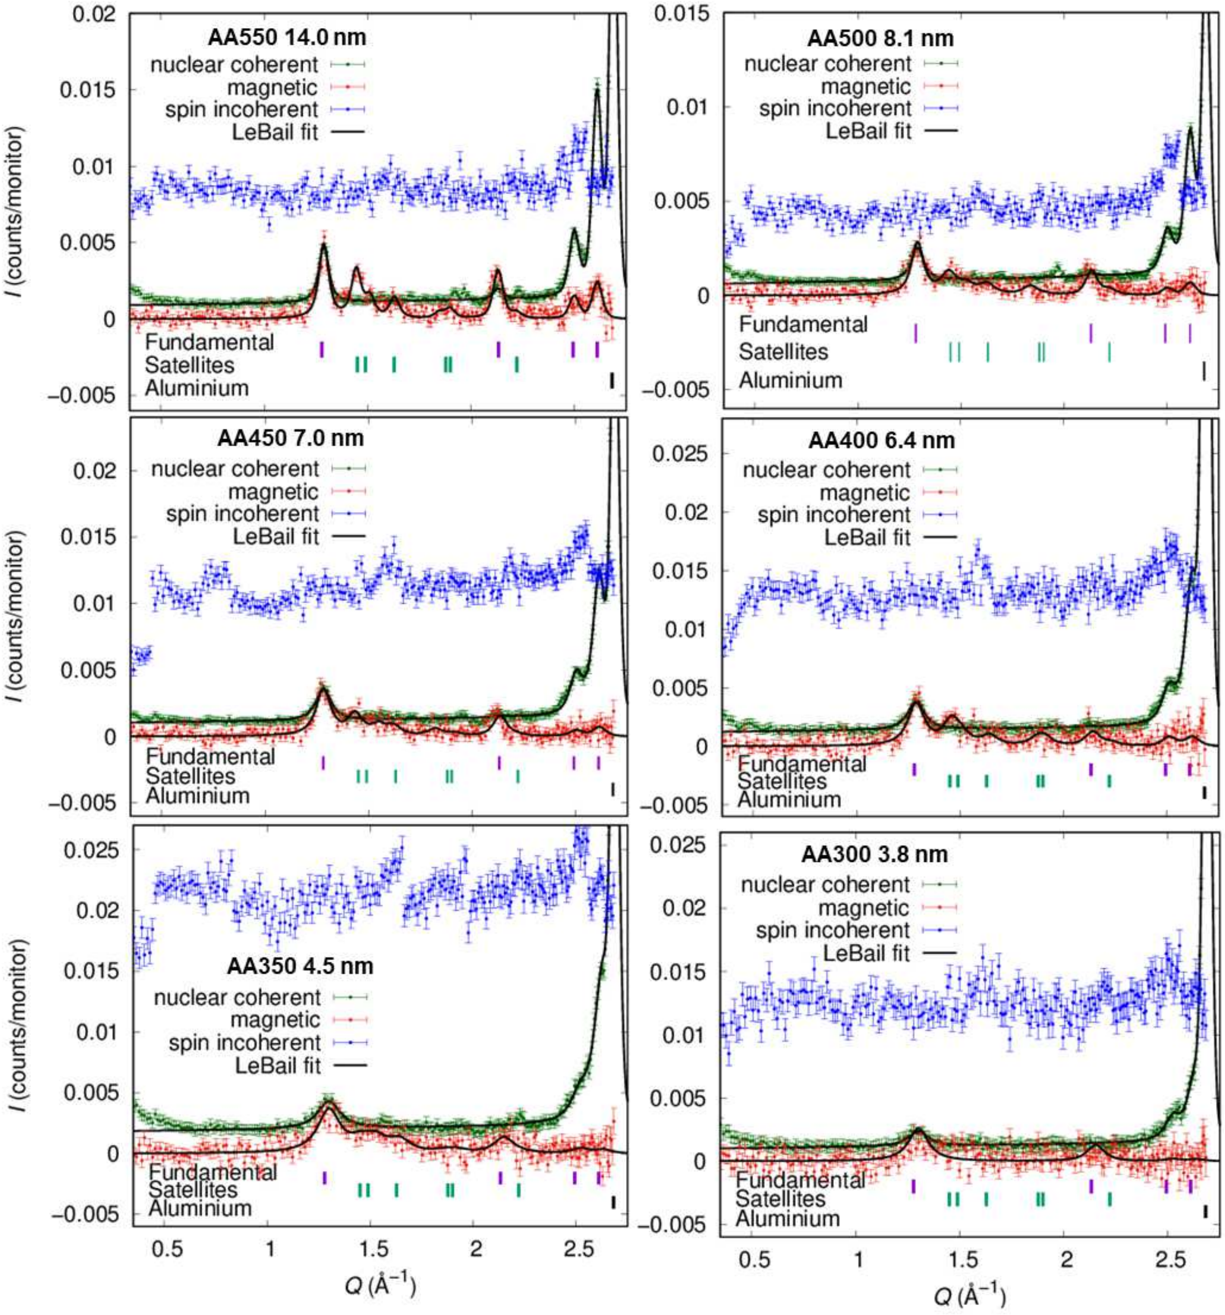


Fig. S 5. Separated neutron scattering contributions of the prepared samples recorded at 3.5 K together with Le-Bail fit. Fundamental magnetic reflection (purple vertical lines) arise from collinear magnetic state, satellite reflections (green vertical lines) are associated to spin-spiral order. The aluminium sample holder gives rise to a reflection at 2.6 Å$^{-1}$.

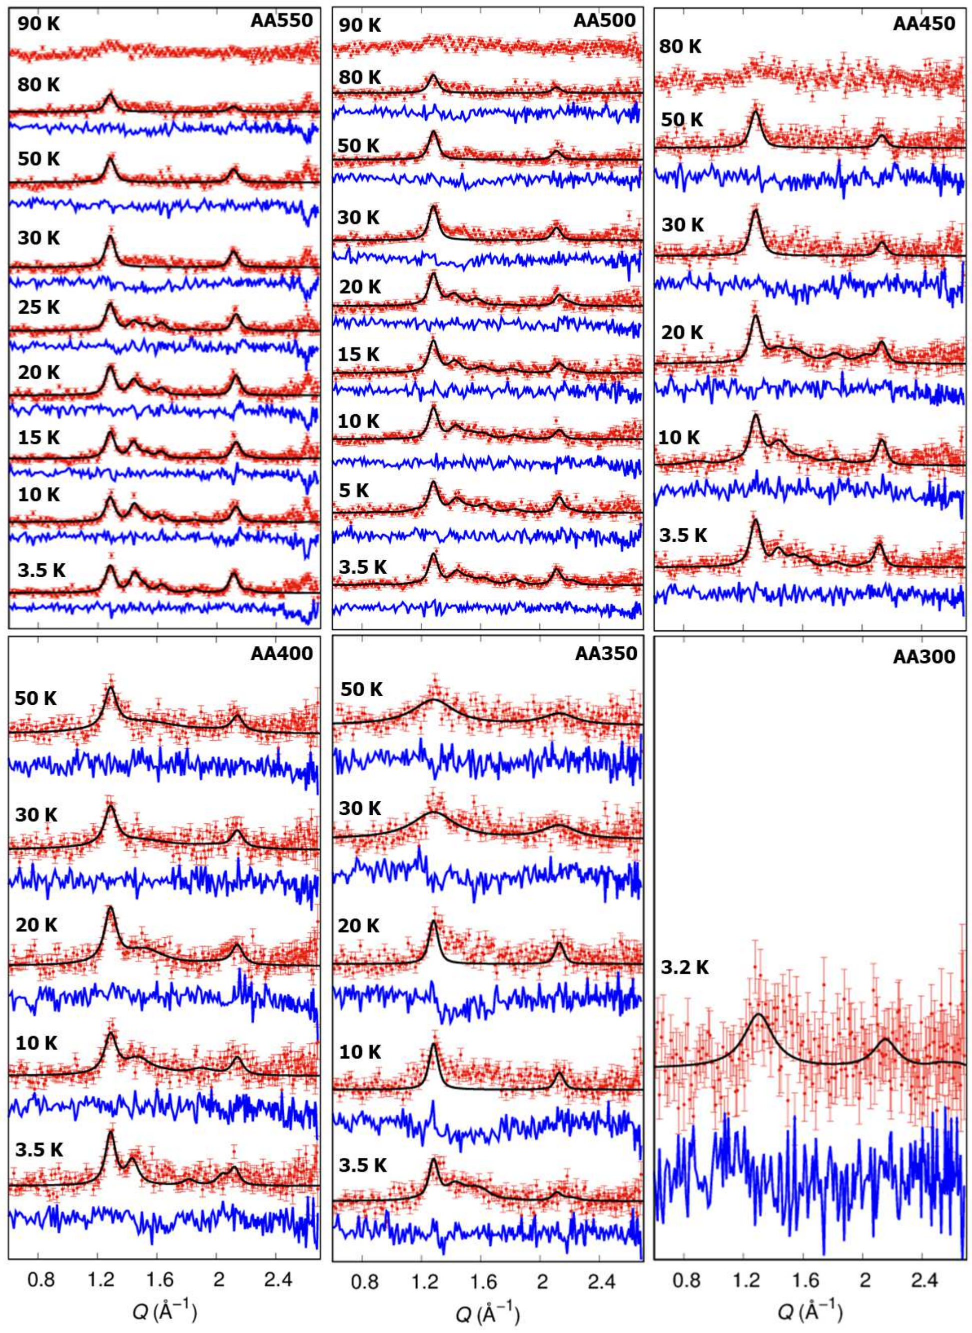


Fig. S 6. Temperature dependence of the magnetic scattering cross section of the prepared cobalt chromite nanoparticles. Red dots display experimental data, the black line is Le-Bail fit and blue line is residual between the fit and experimental data.

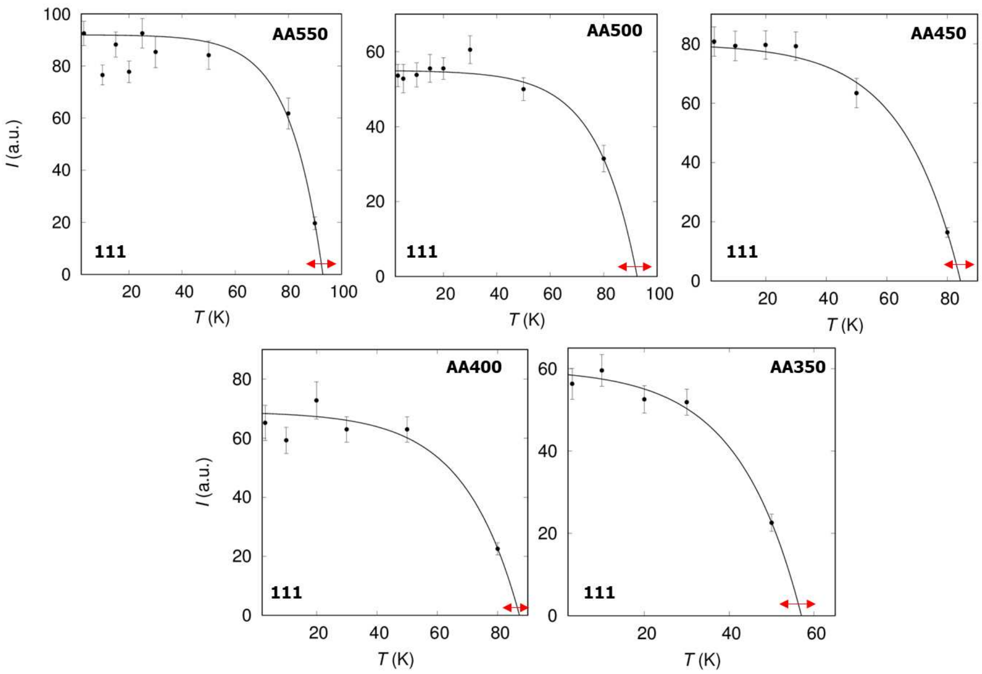


Fig. S 7. Temperature dependence of the (1 1 1) fundamental magnetic reflection intensity. Black line is guide to eye and red double arrow represents the derived $\boldsymbol{\theta}_{\mathrm{C}}$ range.

For AA350, noticeable magnetic satellite reflections only appear at the base temperature 3.5K, which was hence taken as transition temperature.

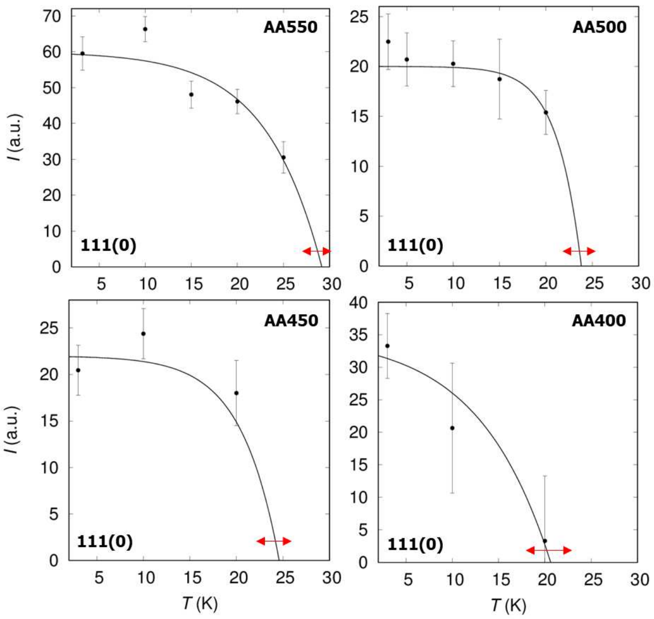


Fig. S 8. Temperature dependence of the (1 1 1 (0)) magnetic satellite reflection intensity. Black line is guide to eye and red double arrow represents the derived $T_\mathrm{s}$ range.

### E. Macroscopic polarization

Due to a large surface to volume ratio in the nanoparticles, contact effects play an important role in direct measurements of the polarization. To circumvent this and clearly see the emergence of the spontaneous polarization at the multiferroic phase transition we chose to observe the polarization by means of higher harmonics measurements of the permittivity[8,9]. Here we exploit that the presence of switchable spontaneous polarization goes along with the onset of non-linear $P(E)$-loops. Thin non-linearity is reflected by the appearance of higher harmonics in the dynamic response to a sinusoidal electric field stimulus: $P(t) = \varepsilon_0 E_{\mathrm{ac}} \sum_{n=1}^{\infty} (\varepsilon_n' \sin n\omega t - \varepsilon_n'' \cos n\omega t)$. Due to the symmetry of a ferroelectric hysteresis loop we expect all contributions for even $n$ to vanish while the odd $n$ should decrease in magnitude by $1/n$. Non-hysteretic contributions from e.g. the interparticle contacts will then only occur in the first harmonic but not in $\varepsilon_3$, the higher harmonic where we expect the largest signal. In **Fig S 9** the result of the measurement with $E_{\mathrm{ac}} \approx 1\,\mathrm{kV/mm}$ at $\nu = 97\,\mathrm{Hz}$ is shown for the sample AA500.

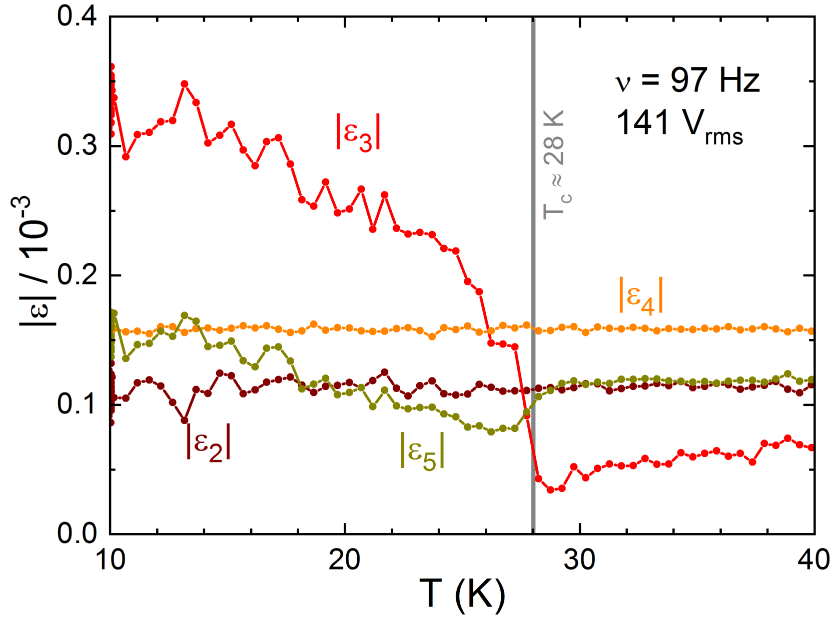


Fig. S 9. Higher harmonic measurements of the permittivity on AA500 show the development of hysteresis in the electric polarization due to transition into the multiferroic phase at $T_c \approx 28\,\mathrm{K}$.

---

* Deceased

† now at: Physics and Materials Science Research Unit, University of Luxembourg, 162A Avenue de la Faencerie, L-1511 Luxembourg, Grand Duchy of Luxembourg

‡ corresponding author: sabrina.disch@uni-koeln.de

[1] D. Zákutná, A. Repko, I. Matulková, D. Nižňanský, A. Ardu, C. Cannas, A. Mantliková, and J. Vejpravová, Journal of Nanoparticle Research **16**, 2251 (2014).

[2] J. Rodriguez-Carvajal, Physica B **192**, 55 (1993).

[3] Y. Su, K. Nemkovskiy, and S. Demirdis, J. Large-Scale Res. Facil. **A27** (2015).

[4] W. Schweika and P. Böni, Physica B **297**, 155 (2001).

[5] A. Glavic, *Plot.py - data plotting and evaluation software*, URL `https://sourceforge.net/projects/plotpy/`.

[6] M.-R. Li, E. McCabe, P. Stephens, M. Croft, L. Collins, S. V. Kalinin, Z. Deng, M. Retuerto, A. S. Gupta, H. Padmanabhan, et al., Nat. Commun. **8**, 2037 (2017).

[7] P. G. Casado and I. Rasines, Polyhedron **5**, 787 (1986), ISSN 0277-5387, URL `http://www.sciencedirect.com/science/article/pii/S0277538700844381`.

[8] D. Niermann, C. Grams, M. Schalenbach, P. Becker, L. Bohatý, J. Stein, M. Braden, and J. Hemberger, Phys. Rev. B **87**, 134412 (2014).

[9] C. Grams, S. Kopatz, D. Brüning, S. Biesenkamp, P. Becker, L. Bohatý, T. Lorenz, and J. Hemberger, Sci. Rep. **9**, 4391 (2019).
